# Supplementary material for: Quantum dynamics of an electromagnetic mode that cannot contain N photons
Source: arXiv:1505.04238 source file (2015-05-19)
Supplement: Supplementary file 1 [file SupmatQZD.pdf]

# Supplementary Materials for

# "Quantum dynamics of an electromagnetic mode that cannot have N photons"

L. Bretheau,[1] P. Campagne-Ibarcq,[1] E. Flurin,[1] F. Mallet,[1] and B. Huard[1]

[1]*Laboratoire Pierre Aigrain, Ecole Normale Supérieure-PSL Research University, CNRS, Université Pierre et Marie Curie-Sorbonne Universités, Université Paris Diderot-Sorbonne Paris Cité, 24 rue Lhomond, 75231 Paris Cedex 05, France*

## I. MATERIAL AND METHODS

### A. Sample fabrication

The superconducting qubit follows the design of the "3D transmon" described in Ref. [11]. A transmon chip is embedded in an empty bulk aluminum cavity of $26.5 \times 26.5 \times 9.5$ mm$^3$, anchored at the base-temperature (20 mK) of a dilution refrigerator. It consists of a single aluminum Josephson junction connected to two antennas of $0.4 \times 1$ mm$^2$ each, aligned along the field polarization of the TE 110 mode and placed at the maximum of the field. The transmon chip was fabricated on a single-crystal C-plane sapphire substrate, using electron-beam lithography followed by aluminum double-angle electron-beam evaporation. Film thickness for each evaporation is approximately 30 nm and 85 nm which takes into account the evaporation angles $\pm 30°$. The two layers are separated by a thin AlOx layer grown in an atmosphere of 20 % $O_2$ and 80 % Ar at 20 mbar for 7 min to form the tunnel junction. This resulted in a room temperature normal state resistance of 4.85 k$\Omega$.

### B. Measurement setup

Figure S1 is a block diagram of the measurement setup. The system is probed through SMA connectors whose central pin dips inside the 3D cavity. Readout and drive pulses are generated by standard single side-band (SSB) modulation of continuous microwave tones. The modulation is performed by mixing continuous waves produced by microwave generators with pulsed sinusoidal signals synthesized by different channels of a Tektronix Arbitrary Waveform Generator (AWG). All sources are synchronized by an atomic clock. The system is always probed through a readout of the qubit, using the qubit-state dependent transmission of the cavity. It is performed by shining a tone at 7.8041 GHz $\simeq f_c$ including the 40 MHz modulation (chosen to optimize the readout). To excite the cavity and realize the displacement pulse, the cavity is driven at $f_c = 7.8037$ GHz, including the 80 MHz modulation. The qubit drives, which are used for both the Hilbert space blockade and the conditional and unconditional pulses of the qubit, are performed at $f_q = 5.622$ GHz including the 200 MHz modulation.

These pulses are sent through an heavily attenuated and filtered input coax line (with cryogenic attenuators at various stages of the dilution refrigerator), ensuring that negligible thermal excitations enter the device. A commercial low-pass filter (from K&L) with 12 GHz cut-off frequency is used at the still stage (850 mK), while a homemade low-pass filter consisting in a microstrip line enclosed in an infrared tight box filled with Eccosorb is inserted at base temperature. Note that a similar line, denoted as "reflection probe" in Fig. S1, has been used for an in situ estimation of cavity input and ouput coupling rates $\Gamma_{in,out}$ , but is unused in the discussed experiment. Finally, the transmon aluminum 3D cavity is enclosed in an infrared tight copper box thermally anchored to the 20 mK stage. Its inside walls are all covered by a radiation absorbing coating consisting of 1 mm diameter SiC grains mixed up in Eccosorb.

Two cryogenic circulators in series are used to direct the readout signal from the cavity toward a Josephson mixer [26] used as a low noise non-degenerate amplifier at cavity frequency $f_c$. It is pumped with a continuous pump tone at 19.6 GHz and realizes a +26 dB gain with 7 MHz bandwidth. A cryoperm magnetic shield encloses the Josephson mixer and its biasing coil (not shown). The output signal of the Josephson amplifier is routed back through a superconducting NbTi coax cable towards a low noise HEMT (High Electron Mobility Transistor) amplifier of 30 dB gain from Caltech University, isolated with a bias-tee and two circulators in series. The signal is further amplified at room temperature and down-converted to 40 MHz before being digitized by a 16-bit ADC at 160 MS.s$^{-1}$ and numerically demodulated using an FPGA (Field Programmable Gate Array) board.

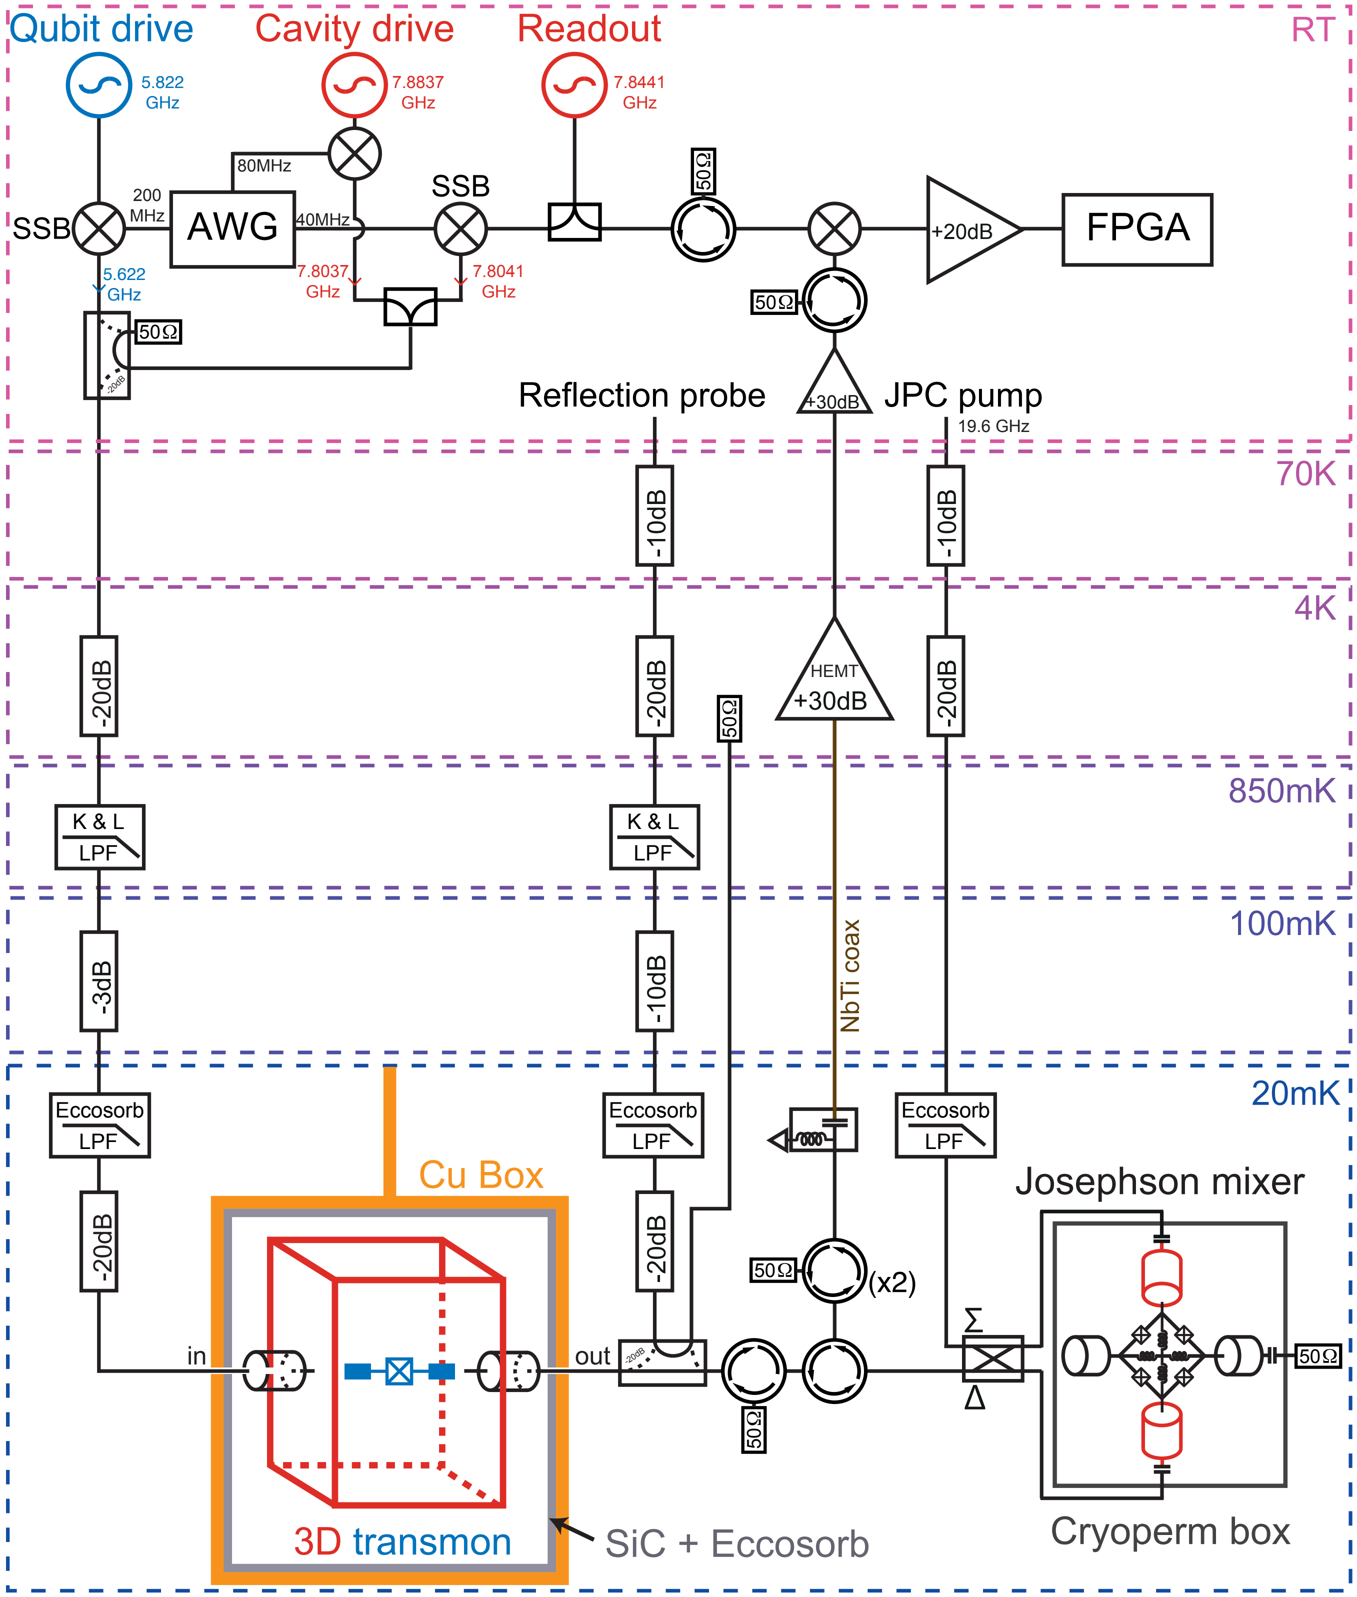


Figure S1: **Schematics of the experimental setup.** Measurement and drive microwave pulses are generated by single sideband (SSB) modulation and sent through the input line, which is heavily attenuated (XMA attenuators) and filtered (K&L and homemade Eccosorb low-pass filters (LPF)). The readout signal transmitted through the 3D cavity is amplified by a Josephson mixer and routed out of the fridge where it is digitized using an FPGA board. The dc line feeding the coil which allows one to flux bias the Josephson mixer is not represented.

## II. MODELING THE CAVITY-QUBIT SYSTEM

### A. Full system Hamiltonian

In the strong dispersive limit, the cavity-qubit system can be described by the Hamiltonian

$$H_T/h = f_c a^\dagger a + f_q|e\rangle\langle e| - \chi a^\dagger a|e\rangle\langle e| - \lambda a^\dagger a^\dagger aa + \beta a^\dagger a^\dagger aa|e\rangle\langle e|, \tag{S1}$$

with $a^\dagger/a$ the raising/lowering operators of the cavity and $|e\rangle$ the excited state of the qubit. The first two terms are each responsible for the cavity and qubit dynamics. The third term describes the first order coupling between the cavity and qubit modes. The resulting state-dependent frequency shift is the basis for both the photon-selective phase space barrier, the mapping of the cavity state onto the qubit state and the qubit readout. The last two terms are two orders of magnitude smaller. The fourth term describes the anharmonicity of the dressed cavity mode, which is supposedly inherited from the Josephson junction. This self-Kerr results in a photon-number dependent cavity frequency. The last term is a non-linear correction to the state dependent shift between the cavity and qubit modes.

### B. Parameter characterization

Figure S2 displays various spectroscopic measurements of the cavity-qubit system. The cavity mode is at $f_c = 7.8037$ GHz when the qubit is in the ground state. Transmission and reflection measurements of the cavity (Fig. S2a and b) allow one to extract the coupling rates to the transmission lines. Neglecting internal losses of the cavity which should be of the order of 2 kHz from previous measurements, one finds $\Gamma_{out} = 100$ kHz and $\Gamma_{in} = 22$ kHz. This results in a photon exit rate $\gamma_c = 2\pi(\Gamma_{out} + \Gamma_{in}) = (1.3\ \mu\text{s})^{-1}$. When the qubit gets excited, the cavity frequency is at $f_c - \chi$, where $\chi = 4.63$ MHz is the frequency shift due to the dispersive interaction with the qubit. The corresponding resonance is visible in Fig. S2c due to the 22 % thermal population of the qubit [27].

Symmetrically, and as seen in Fig. S2d, the qubit frequency depends on the photon number $k$ in the cavity as $f_q - k\chi$, with $f_q = 5.622$ GHz the qubit frequency when the cavity is in the ground state. With this measurement, which is a spectroscopy of the qubit in presence of a coherent state, one can resolve the photon number states [10]. The bare qubit frequency $f_q$ differs from the next transition by an anharmonicity $\alpha = 172.5$ MHz. The measured qubit relaxation time is $T_1 = 11.52\ \mu$s, and the Ramsey time is $T_2 = 8.9\ \mu$s.

### C. Anomalous Kerr effect

Higher order interaction terms are visible in Fig. S2. In particular, the cavity frequency depends on the average photon number in the cavity (Fig. S2c). Strikingly, it increases when the photon number increases, which is in contradiction to all reported transmon qubits and 3D transmon models such as those in Refs. [14–16]. Here, the corresponding self-Kerr frequency is estimated to be $\lambda = -70$ kHz from a fit of the Wigner functions time evolution. Similarly, Fig. S2d shows that the qubit frequency for each Fock state $|k\rangle$ increases with the overall average photon number, which is also opposite to what is usually seen [10, 28]. At last, the frequency $\beta$ can be extracted from a further measurement and one gets $\beta = -23$ kHz, which is also opposite to what has been previously measured [19].

We want to stress that during the first cool-down of the sample, these Kerr terms were initially positive and of similar amplitude [29]. They became negative after an unwanted warm-up (around 270 K) and cool-down of the fridge that barely modified the other parameters. Understanding the origin of these exotic "negative Kerr" terms might allow one to design a qubit-cavity system with a very small anharmonicity for the cavity.

### D. Numerical simulation of the cavity field dynamics

The Hamiltonian in Eq. (1) of the main text, which only describes the cavity dynamics, is obtained by projecting the qubit onto the ground state in Eq. (S1). In order to model the blockade at level $N$, the annihilation operator $a$ is replaced by an effective annihilation operator

$$a_N = a - \sqrt{N}|N-1\rangle\langle N| - \sqrt{N+1}|N\rangle\langle N+1|, \tag{S2}$$

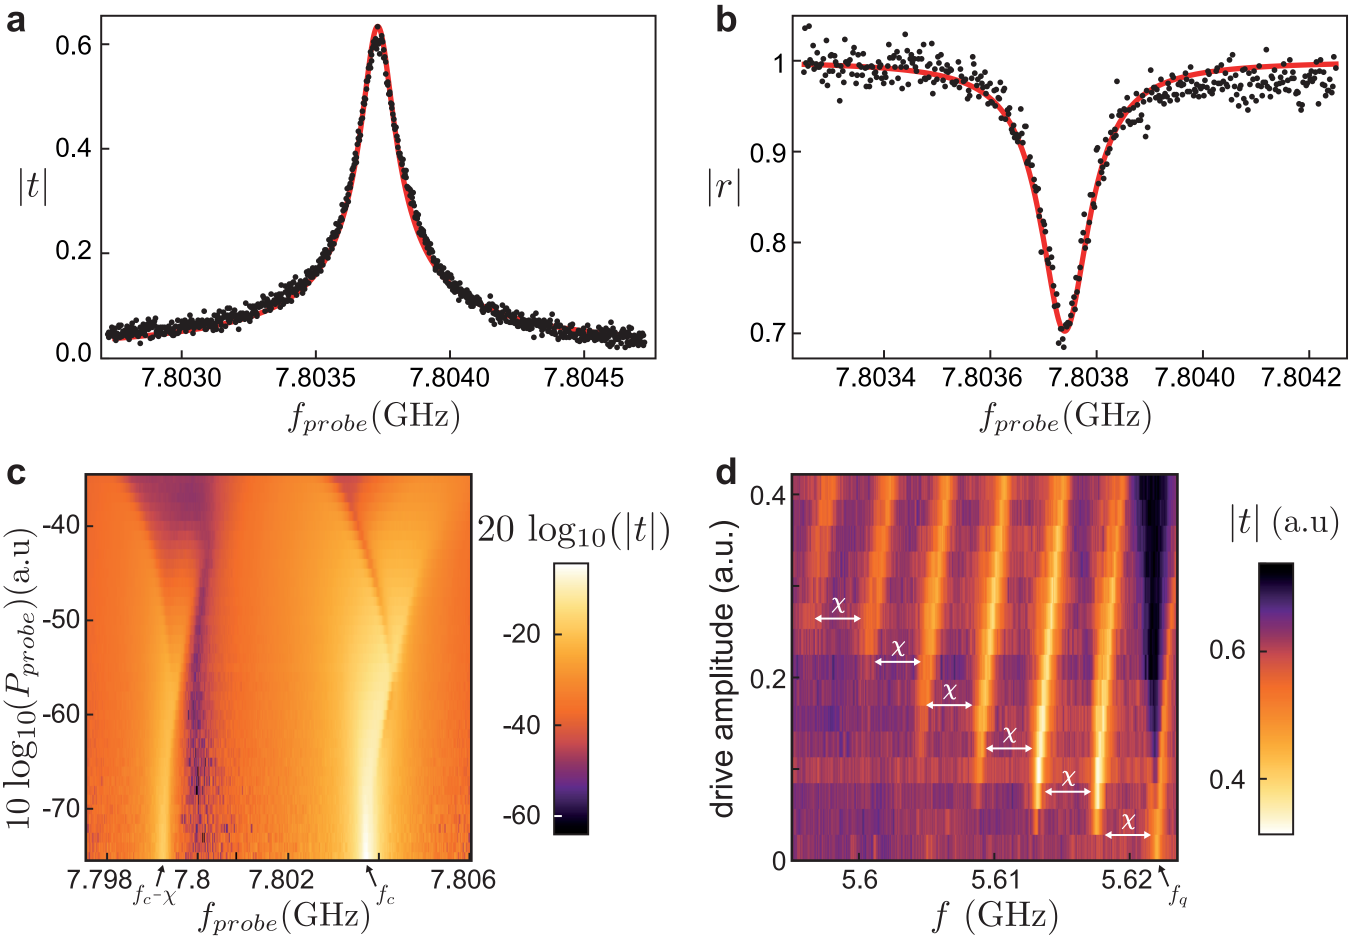


Figure S2: **Cavity-qubit characterization. a, b** Measured (black dots) and predicted (solid red line) transmission $|t|$ (**a**) and reflexion $|r|$ (**b**) of the cavity as a function of frequency at low power. The measurements include the unknown overall transmission and reflexion of the setup so that they are scaled with a proportionality factor to fit with theory. The reflected signal is obtained using the reflection probe shown in Fig. S1. **c,** Measured transmission $|t|$ of the cavity as a function of both frequency and input power. Qubit is at thermal equilibrium before measurement. The resonance at $f_c$ (respectively $f_c - \chi$) corresponds to the qubit being in the ground (resp. excited) state. When the input power increases, the resonances shifts to higher frequency, due to an anomalous Kerr effect. **d,** Shown are qubit spectra with coherent cavity drive at different amplitudes. The 50 $\mu$s long excitation pulse at frequency $f$ is performed while the cavity is driven at its resonance frequency $f_c$ with a given amplitude. After waiting 2 $\mu$s to let the field leak out of the cavity, the qubit state is probed by measuring the transmission $|t|$ (encoded in color) of the cavity at a frequency close to $f_c$. The spectra have resolved peaks corresponding to each photon number, separated by $\chi = 4.63$ MHz. As the amplitude of the cavity drive increases, the average cavity occupation gets higher and more Fock states are resolved. The observed shift of qubit frequency with average photon number is related to the Kerr-term.

for which transitions involving N photons are removed. The Hamiltonian contains an additional term which takes into account an external drive at frequency $f_d$. In the rotating frame at the drive frequency $f_d$, it reads

$$H = h(f_c - f_d)a_N^\dagger a_N - h\lambda a_N^\dagger a_N^\dagger a_N a_N + i\hbar\epsilon_d(a_N^\dagger - a_N). \tag{S3}$$

The evolution of the field can be modeled using the Master equation for the field density matrix $\rho$

$$\partial_t \rho = -\frac{i}{\hbar}[H,\rho] + \frac{\gamma_c}{2}(2a\rho a^\dagger - \rho a^\dagger a - a^\dagger a \rho), \tag{S4}$$

The first term in Eq. (S4) describes the standard Hamiltonian evolution. The second one, which has the Lindblad form, encodes cavity relaxation. Note that the standard annihilation operator $a$ remains in Eq. (S4) since QZD is not effective against relaxation.

All the theoretical results presented in the main text are obtained by numerical resolution of Eq. (S4) in a 15-dimensional truncated Hilbert space. This is done by using "QuTip", a Quantum toolbox for Python [30]. Using

this model, one can reproduce with a good agreement both the photon number probabilities $\tilde{P}_k$ and the Wigner function $W(\alpha)$ shown in Fig. 2,3 and 4 of the main text. The drive amplitude $\epsilon_d$ and detuning $f_c - f_d$, and the cavity anharmonicity $\lambda$ are chosen to optimally match the measurements. The amplitude of the drive $\epsilon_d$, which directly determines the period of the oscillations in the occupation is finely tuned between 2.83 and 3.05/$\mu$s for each blocked level $N$. The anharmonicity $\lambda = -70$ kHz is found to be negative, in agreement with measurements of Fig. S2. At last, we attribute the origin of the detuning $f_c - f_d$ to an energy shift of the levels due to the blocking tone. It was found to be $-0.1$ MHz for $N > 2$ and $-0.4$ MHz for $N = 2$. These values are consistent with the system being more strongly disturbed by the blocking field at $N = 2$ than for larger $N$.

## III. MEASUREMENT SCHEMES

In the experiment, the state of the cavity mode is determined by entangling the cavity with the ancillary qubit and then measuring the qubit state. Since the qubit state is readout using the qubit-state dependent transmission of the very same cavity, we always wait 2 $\mu$s after "mapping" the cavity state onto the qubit state to empty the cavity. The qubit state is then detected by shining a tone at the cavity frequency $f_c$ and integrating the transmitted signal during 6 $\mu$s. The frequency and power of the readout pulse were optimized to improve the measurement rate.

In practice, we have used two different methods to characterize the state of the cavity field. We either measure the diagonal elements of its corresponding density matrix, i.e. the Fock state probabilities, or we measure the full density matrix through a direct Wigner tomography.

### A. Measuring Fock state probabilities

#### *1. Conditional qubit rotations*

To measure the Fock state distribution of any arbitrary field state stored in the cavity, we perform conditional rotations of the qubit. To do so, we use the fact that the qubit transition frequency is dependent on the photon number state of the resonator, through the term $-h\chi a^\dagger a\sigma_z$. In practice, we apply a 0.4 $\mu$s $\pi$-pulse at frequency $f_q - k\chi$. Its duration is much longer than $\chi^{-1}$ to ensure its selectivity in photon number, and shorter than $\gamma_c^{-1}$ to minimize cavity relaxation. The pulse is shaped with a gaussian envelope of characteristic spectral bandwidth $\sigma = 2.1$ MHz. This results in a pulse selectivity $1 - e^{-\frac{\chi^2}{2\sigma^2}} > 0.9$. As depicted in Fig. S3a, such a conditional rotation corresponds to a CNOT operation on the qubit, conditioned on the photon number in the cavity [12].

This procedure entangles the qubit and cavity states. If the qubit is initially in the ground state, the qubit gets excited by this operation if and only if $k$ photons are in the cavity. Measuring the probability to find the qubit in the excited state hence gives the probability $P_k = \mathrm{Tr}(\rho|k\rangle\langle k|)$ for the field to be in Fock state $|k\rangle$.

#### *2. Determination of the Fock state probabilities of a coherent state*

To test this procedure, we have used it to measure the Fock state probabilities of the coherent state created by the displacement $D(\alpha)$ used in the Wigner tomography. Incidentally, this allowed us to calibrate $D(\alpha)$. Right after the displacement, a photon selective $\pi$-pulse at frequency $f_q - k\chi$ is applied to the qubit and the qubit state is measured after waiting 2 $\mu$s.

The corresponding transmitted signal is shown in Fig. S3b as a function of the amplitude of the displacement pulse, for $k$ ranging from 0 to 6. Two spurious effects have to be considered to infer the Fock state probabilities $\tilde{P}_k$.

First, the transmission depends on the displacement amplitude due to the cavity anharmonicty (self-Kerr). To get rid of this effect, we always perform a control measurement without any qubit rotation (black-dotted curve), which is subtracted to the signal of interest (color-dotted curves).

Second, the qubit has a residual thermal population and about $p_e = 22$ % of the experiments start with a qubit in the excited state. In these cases, the displacement is not effective and the system remains in $|0, e\rangle$. This affects the signal for $k = 0$ (red-dotted curve) which is above all the other curves at large drive amplitude (Fig. S3b). At such a large displacement amplitude, the probability of being in state $|g, 0\rangle$ is very small and the selective $\pi$-pulse is efficient only when the qubit was initially thermally excited. In this case, it empties state $|e, 0\rangle$ in state $|g, 0\rangle$. This phenomenon can actually be used as a procedure to cool the qubit [31]. In contrast, state $|e, 0\rangle$ stays occupied for $k \geq 1$.

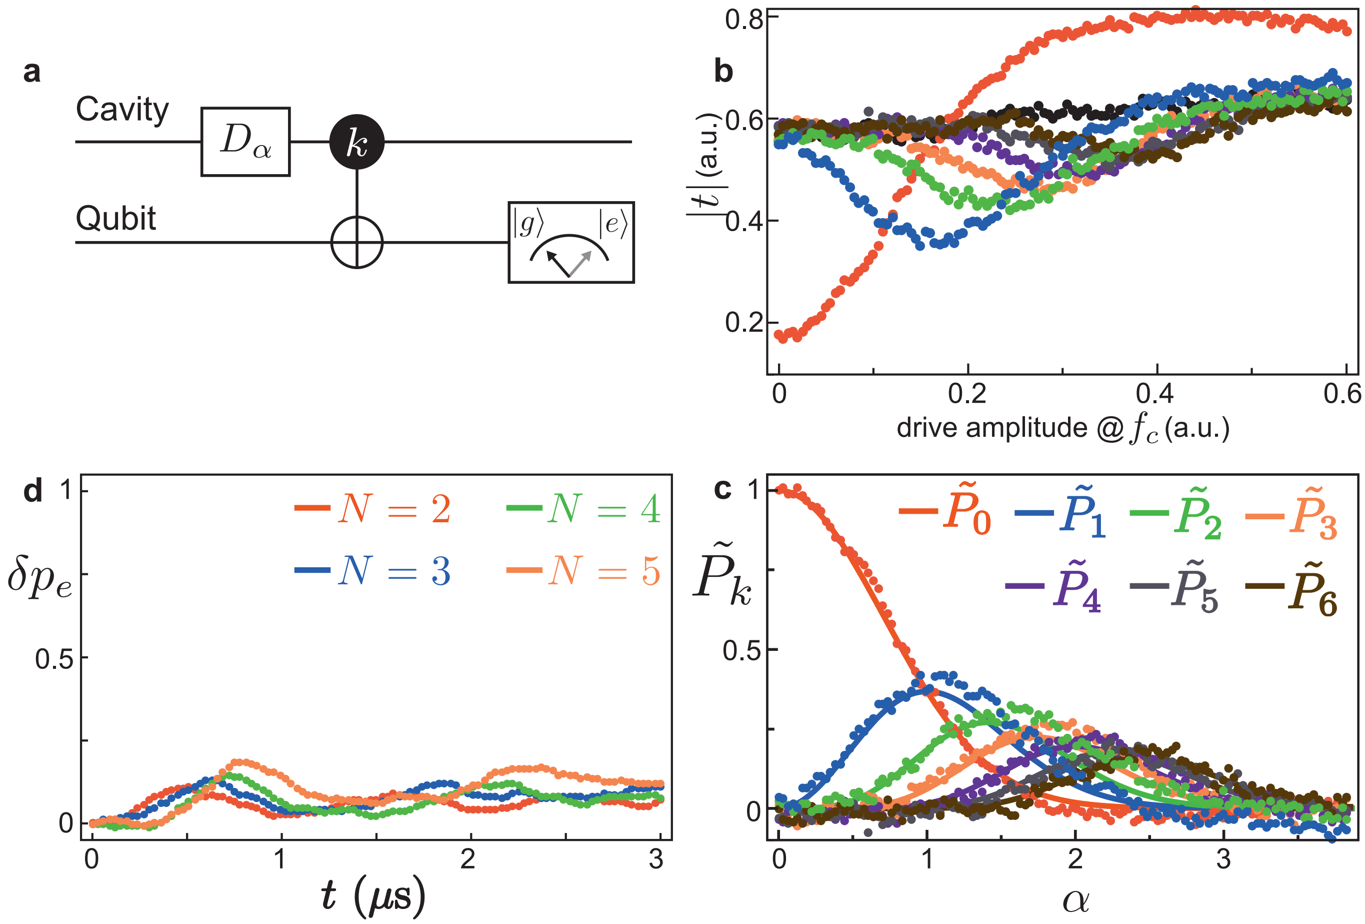


Figure S3: **Measuring Fock state probabilities.** **a**, Circuit diagram for detecting the Fock state probability $P_k$ as a function of the coherent displacement $\alpha$. After a 240 ns displacement pulse at $f_c$, a conditional qubit rotation is applied to the qubit so that it is excited if and only if $k$ photons are in the cavity. After a 2 $\mu$s waiting time to empty the cavity, the qubit state is measured using the qubit-state dependent transmission of the cavity. **b**, Shown is the corresponding transmission $|t|$ of the cavity at frequency $f_c$ as a function of drive amplitude for different values of $k$ (encoded in color from 0 to 6, as labeled in c below). The black curve, which corresponds to the case without any qubit rotation, depends slightly on the drive amplitude due to the self-Kerr effect of the cavity. **c**, Measured (dots) and theoretical (solid lines) Fock state probabilities $\tilde{P}_k$ as a function of the coherent displacement $\alpha$. The axes were scaled to fit a Poisson distribution $P_k(\alpha) = e^{-|\alpha|^2}\frac{|\alpha|^{2k}}{k!}$ (solid lines) with three free fit parameters to all seven Fock state populations simultaneously. This allows one to calibrate the drive amplitude in term of coherent displacement $\alpha$. **d**, Shown is the additional probability of being in the qubit excited state as a function of time, in presence of both blocking tone at level $2 \leq N \leq 5$ and coherent drive. This leak is taken into account to infer an effective Fock state probability $\tilde{P}_k$ in the main text.

Starting from thermal equlibrium and under a resonant drive at frequency $f_c$, a field develops only if the qubit is in $|g\rangle$ since the cavity is out of resonance when the qubit is in $|e\rangle$. The system is then in the state

$$\rho_{T,ref} = (1 - p_e)|\psi\rangle\langle\psi| \otimes |g\rangle\langle g| + p_e|0\rangle\langle 0| \otimes |e\rangle\langle e|, \tag{S5}$$

with $|\psi\rangle = \sum_n c_n|n\rangle$ the cavity state corresponding to the qubit initially in $|g\rangle$. The associated reference signal is

$$S_{ref} = (1 - p_e)\sum_n \tilde{P}_n t_{n,g} + p_e t_{0,e} \tag{S6}$$

with $t_{n,g}$ ($t_{n,e}$) the transmission for the qubit in the ground (excited) state and $n$ photons in the cavity, and $\tilde{P}_n = |\langle n|\psi\rangle|^2 = |c_n|^2$ the probability of finding $n$ photons knowing that the qubit is initially in $|g\rangle$. These probabilities are precisely what we want to extract. To that aim, one needs to apply, for each value of $k$, a pulse at frequency $f_q - k\chi$.

After this $\pi$-pulse conditioned to Fock state $k$, the system is in the state

$$\rho_{T,k} = (1 - p_e)|\psi_{k,g}\rangle\langle\psi_{k,g}| + p_e|\psi_{k,e}\rangle\langle\psi_{k,e}| \tag{S7}$$

with

$$\begin{cases} |\psi_{k,g}\rangle = \sum_{n\neq k} c_n|n\rangle \otimes |g\rangle + c_k|k\rangle \otimes |e\rangle \\ |\psi_{0,e}\rangle = -|0\rangle \otimes |g\rangle \\ |\psi_{k\neq 0,e}\rangle = |0\rangle \otimes |e\rangle \end{cases} \tag{S8}$$

Then, the measured signal is

$$S_k = (1-p_e)\left[\tilde{P}_k t_{k,e} + \sum_{n\neq k} \tilde{P}_n t_{n,g}\right] + \begin{cases} p_e t_{0,g}, & \text{if } k = 0 \\ p_e t_{0,e}, & \text{if } k \neq 0 \end{cases}. \tag{S9}$$

By subtracting the two signals, it is possible to isolate the contribution of the $k$-th level from all the other levels. Indeed,

$$\tilde{S}_k = S_{ref} - S_k = \tilde{P}_k \times (1-p_e)\,(t_{k,g} - t_{k,e}) - \delta_{k,0} p_e\,(t_{0,g} - t_{0,e}) \tag{S10}$$

with $\delta$ the Kronecker delta.

Therefore, the Fock state probability is given by

$$\tilde{P}_k = \frac{\tilde{S}_k}{(1-p_e)\,(t_{k,g} - t_{k,e})} + \delta_{k,0}\frac{p_e}{1-p_e}. \tag{S11}$$

The nonzero thermal population $p_e$ of the qubit only induces an offset in the probability of measuring 0 photon (second term). With no prior knowledge of the qubit state (apart from its statistical population) and without performing any post-selection, one thus accesses the conditional probability of occupying level $k$ on the condition that the qubit is initially in the ground state.

We have used this procedure with $p_e$ =0.22 and $t_{k,g} - t_{k,e} = t_{0,g} - t_{0,e} = 0.3955$, which were adjusted such that $\tilde{P}_0 = 0$ at large drive amplitude and $\tilde{P}_0 = 1$ in the ground state at zero displacement [13]. In order not to add extra noise, we don't subtract directly $S_{ref}$ but rather its third order polynomial fit. The inferred Fock state probabilities are shown as dotted lines in Fig. S3c. The solid lines correspond to the standard Poisson distribution of a coherent state

$$\tilde{P}_k(\alpha) = e^{-|\alpha|^2}\frac{|\alpha|^{2k}}{k!}. \tag{S12}$$

The overall agreement validates the hypothesis of a $k$-independent scaling amplitude, i.e. a linear readout (see Supplementary Information in Ref [12]).

This measurement and comparison with theory allows us to calibrate the drive amplitude of the displacement pulse in square root of photons. This independent calibration was used to scale the axis of the different Wigner tomographies shown in the main text. Besides, this measurement also demonstrates that the fast displacement pulse shaped with DRAG technique indeed produces a coherent state only when the qubit is in the ground state, and that one can safely ignore any Kerr distortion with so short pulses.

### *3. Determination of the Fock state probabilities of a field under QZD*

In presence of both blocking tone at level $N$ and coherent drive, we observe a parasitic excitation of the qubit. This additional excitation $\delta p_e$ is independently measured in time and remains below 18 % (see Fig. S3d). This measurement is obtained by measuring the transmission at the cavity frequency, in absence of any $\pi$-pulse

$$S_{ref}(t) = (1 - p_e - \delta p_e(t))\sum_n \tilde{P}_n t_{n,g} + (p_e + \delta p_e(t))\,t_{0,e}. \tag{S13}$$

The leak into the excited state is therefore given by

$$\delta p_e(t) = \frac{S_{ref}(0) - S_{ref}(t)}{\sum_n \tilde{P}_n (t_{n,g} - t_{0,e})} \simeq \frac{S_{ref}(0) - S_{ref}(t)}{t_{0,g} - t_{0,e}}. \tag{S14}$$

Here, we neglect the dependence of the transmission on the photon number due to the self-Kerr effect. This is reasonable since one remains at low photon number in presence of Hilbert space blockade.

However, this measurement corresponds to the total extra excitation in state $|e\rangle$ and $\delta p_e(t)$ is not resolved in Fock state. Assuming all levels $|k\rangle \otimes |e\rangle$ to be equally excited for $0 \leq k < N$ (on top of the thermal excitation), one can infer the effective probability to be in Fock state $|k\rangle$

$$\tilde{P}_k \leftarrow \tilde{P}_k + \frac{2\delta p_e}{N(1-p_e)}, \text{ for } 0 \leq k < N. \tag{S15}$$

The corresponding probabilities are shown in Fig. 2 of the main text.

Note that the origin of this leak from ladder $|g\rangle$ to ladder $|e\rangle$ is not fully understood. It might be related to the fact that the amplitude of the blockade, which is characterized by the Rabi frequency $\Omega_R$, is of the order of the dispersive shift $\chi$, such that the blocking tone is not perfectly selective in $N$. To improve this aspect, one would need to design a cavity-qubit system with a larger difference between $\gamma_c$ and $\chi$, while keeping the cavity anharmonicity $\lambda$ smaller than $\gamma_c$. Thus, one could choose a Rabi frequency such that $\lambda < \gamma_c \ll \Omega_R \ll \chi$. Yet, a simple model where $p_{k,e}$ comes from detuned Rabi oscillations fails to reproduce our results.

## B. Wigner tomography

### 1. *Conditional displacement pulse and unconditional qubit rotation*

The Wigner function is defined as $W(\alpha) = \mathrm{Tr}(D_\alpha^\dagger \rho D_\alpha \mathcal{P})$, where $D_\alpha = e^{\alpha a^\dagger - \alpha^* a}$ is the field displacement operator and $\mathcal{P} = e^{i\pi a^\dagger a}$ the photon parity operator. Measuring the Wigner distribution of a field therefore amounts to measuring the average photon parity of the field displaced by an amplitude $\alpha$.

The procedure, which is described in the main text, is schematized in Fig. S4a. It requires to be able to perform fast displacement of the cavity and broadband qubit rotation so as to succeed independently of the cavity state.

The displacement is performed by sending a 240 ns pulse at the cavity frequency $f_c$. The pulse is shaped using the DRAG technique [32], which consists in adding to a pulse $\mathcal{A}(t)$ its second derivative in time $\mathcal{A} + \Delta^2 \partial_t^2 \mathcal{A}$. The proportionality factor $\Delta$ is chosen such that the overall Fourier transform cancels at frequencies $f_c \pm \Delta$. With $\Delta = \chi$, it prevents the field to enter in the cavity when the qubit is in its excited state (at frequency $f_c - \chi$). In practice we have used a Gaussian pulse for $\mathcal{A}$ with a 67 ns full width at half maximum.

The qubit rotation is performed by shining a 50 ns broadband pulse at the qubit frequency $\nu_q$. We have used a "sinc" shape and a gaussian envelope to design a bandwidth larger than $10\chi$. At the photon level considered in the experiment ($k < 10$), this $\pi/2$-rotation of the qubit can be regarded as unconditional.

### 2. *Qubit state revival using Ramsey interferometry*

This procedure was calibrated with the vacuum state as initial state, and for various waiting $\tau$. Starting from the ground state, the field is displaced by an amplitude $\alpha$. The total density matrix describing the cavity-qubit system is

$$\rho_T(0) = (1-p_e)|\alpha\rangle\langle\alpha| \otimes |g\rangle\langle g| + p_e|0\rangle\langle 0| \otimes |e\rangle\langle e|, \tag{S16}$$

with $|\alpha\rangle = e^{-\frac{|\alpha|^2}{2}} \sum_{k=0}^{\infty} \alpha^k |k\rangle/\sqrt{k!}$ the coherent state of amplitude $\alpha$. The displacement is fast enough so that the state is coherent despite Kerr terms.

Then, one applies a broadband $\pi/2$ pulse, lets the qubit evolve during a time $t$ and applies another broadband $\pm\pi/2$ pulse (see Fig. S4a). In practice, two types of experiments are performed with a final pulse either $+\pi/2$ or $-\pi/2$. At the end of this Ramsey sequence, the density matrix is

$$\rho_{T,\pm}(t) = (1-p_e)|\psi_{g,\pm}\rangle\langle\psi_{g,\pm}| + p_e|\psi_{e,\pm}\rangle\langle\psi_{e,\pm}|, \tag{S17}$$

with

$$\left\{ \begin{array}{ll} |\psi_{g,\pm}\rangle & = R_{y,\pm\frac{\pi}{2}} e^{i2\pi\chi t a^\dagger a |e\rangle\langle e|} R_{y,\frac{\pi}{2}} |\alpha\rangle \otimes |g\rangle \\ |\psi_{e,\pm}\rangle & = R_{y,\pm\frac{\pi}{2}} e^{i2\pi\chi t a^\dagger a |e\rangle\langle e|} R_{y,\frac{\pi}{2}} |0\rangle \otimes |e\rangle \end{array} \right. \tag{S18}$$

and $R_{y,\theta} = \exp(-i\frac{\theta}{2}\sigma_y)$. One finds

$$\left\{ \begin{array}{ll} |\psi_{g,\pm}\rangle & = \frac{1}{2}\left(|\alpha\rangle \mp |\alpha e^{i2\pi\chi t}\rangle\right) \otimes |g\rangle + \left(\pm|\alpha\rangle + |\alpha e^{i2\pi\chi t}\rangle\right) \otimes |e\rangle \\ |\psi_{e,+}\rangle & = -|0\rangle \otimes |g\rangle \\ |\psi_{e,-}\rangle & = |0\rangle \otimes |e\rangle. \end{array} \right. \tag{S19}$$

After this Ramsey sequence, the transmitted signal, measured at the cavity frequency is

$$\begin{cases} S_+ = \frac{1}{4}(1-p_e)e^{-|\alpha|^2}\sum_k \frac{|\alpha|^{2k}}{k!}\left[\left(2-e^{i2\pi k\chi t}-e^{-i2\pi k\chi t}\right)t_{k,g}+\left(2+e^{i2\pi k\chi t}+e^{-i2\pi k\chi t}\right)t_{k,e}\right]+p_e t_{0,g} \\ S_- = \frac{1}{4}(1-p_e)e^{-|\alpha|^2}\sum_k \frac{|\alpha|^{2k}}{k!}\left[\left(2+e^{i2\pi k\chi t}+e^{-i2\pi k\chi t}\right)t_{k,g}+\left(2-e^{i2\pi k\chi t}-e^{-i2\pi k\chi t}\right)t_{k,e}\right]+p_e t_{0,e}. \end{cases} \tag{S20}$$

Therefore, the differential signal is

$$S_- - S_+ = \frac{1}{2}(1-p_e)e^{-|\alpha|^2}\sum_k \frac{|\alpha|^{2k}}{k!}\left[\left(e^{i2\pi k\chi t}+e^{-i2\pi k\chi t}\right)(t_{k,g}-t_{k,e})\right]-p_e\left(t_{0,g}-t_{0,e}\right). \tag{S21}$$

Assuming a linear readout $t_{k,g}-t_{k,e}=t_{0,g}-t_{0,e}$, the reduced signal, defined similarly to Eq. (S11), is

$$S(\alpha,t)=\frac{S_- - S_+}{(t_{0,g}-t_{0,e})(1-p_e)}+\frac{p_e}{1-p_e}=\exp\left[|\alpha|^2\left(\cos(2\pi\chi t)-1\right)\right]\cos\left[|\alpha|^2\sin(2\pi\chi t)\right]. \tag{S22}$$

This measurement is performed differentially in order to avoid spurious effects due to the cavity anharmonicity (see Supplementary Information in Ref [12]).

Fig. S4 displays the corresponding measurements (b and c) and theory (d). After a time $t_{revival}=\chi^{-1}=216$ ns, there is a revival in the Ramsey signal. This is in agreement with the spectroscopic measurement $\chi=4.63$ MHz. As time increases, there is a reduction in revival visibility partly due to qubit dephasing and to cavity relaxation at large displacements.

At last, one can notice a shift of the revival time as a function of displacement amplitude in the experiment (Fig. S4c), not visible in theory (Fig. S4d). Following Ref. [19], we model this effect by the higher order interaction term $\beta a^\dagger a^\dagger aa|e\rangle\langle e|$ in the Hamiltonian (S1). To first order, this non-linearity results in a small change in the revival time

$$\begin{aligned} t_{revival} &= \frac{1}{\chi}\left(1+\langle a^\dagger a\rangle\frac{\beta}{\chi}\right) \\ &= \frac{1}{\chi}\left(1+|\alpha|^2\frac{\beta}{\chi}\right) \text{ for a coherent state.} \end{aligned} \tag{S23}$$

Fitting the experimental revival time (dashed line in Fig. S4c), one finds a non-linear frequency $\beta=-23$ kHz. Like the cavity self-Kerr anharmonicity $\lambda$, this term is opposite to what has been previously observed [19].

### *3. Wigner function normalization*

In the experiment, the initial state of the cavity is unknown and one wants to make its tomography. To measure the photon parity, we chose a waiting time $\tau=1/2\chi=108$ ns such that the evolution operator is $\exp(i\pi a^\dagger a|e\rangle\langle e|)$. The experimental Wigner function can therefore be defined as $W(\alpha)=S(\alpha,(2\chi)^{-1})$. Note that the thermal population of the qubit and the uncalibrated cavity transmission simply induce a scaling and an offset in the Wigner distributions. In practice, for each Wigner distribution, the zero was defined as the integral far outside the exclusion circle and a scaling factor was applied to normalize the integral of the distribution.

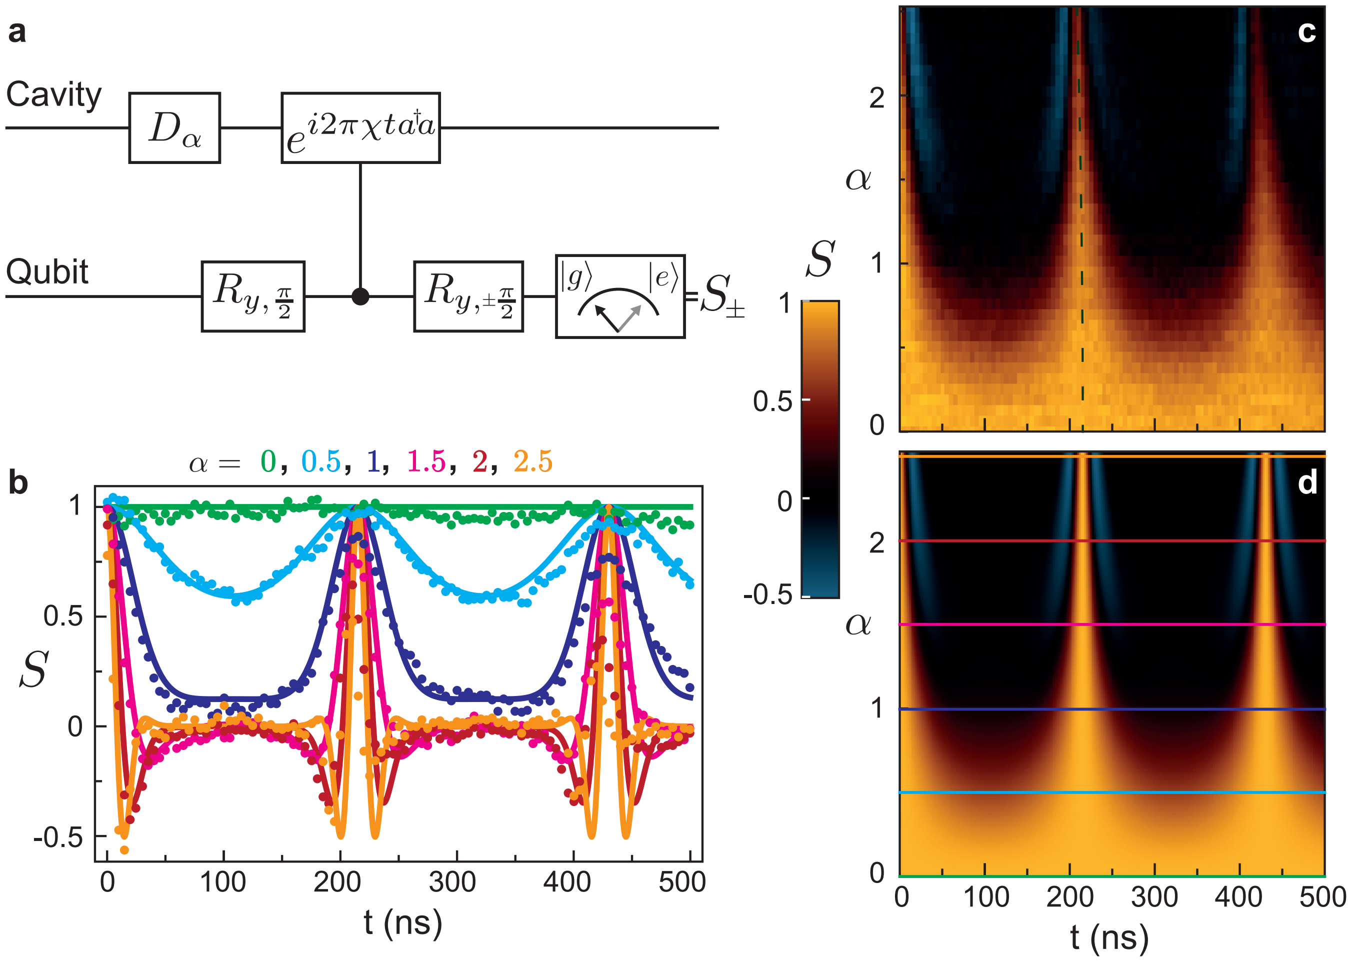


Figure S4: **Qubit state revival using Ramsey interferometry a,** Circuit diagram for Ramsey interferometry of a coherent state under dispersive interaction. After a 240 ns displacement pulse at the cavity frequency, an unconditional $\pi/2$ rotation is applied to the qubit so that it gets in state $(|g\rangle + |e\rangle)/\sqrt{2}$ whatever the cavity state is. Then, one lets the qubit evolve during a time $t$ and performs a second unconditional $\pm\pi/2$ rotation. Finally, after a 2 $\mu$s waiting time to empty the cavity, one measures the qubit state using the qubit-state dependent transmission of the cavity. **b,** Measured (dots) and predicted (lines) signal $S$ as a function of delay time $t$ for various displacement amplitudes $\alpha$. Qubit state revival occurs at a waiting time $t_{revival} = \chi^{-1}$. **c,** Measured signal $S$ as a function of both delay time $t$ and displacement amplitude $\alpha$. At larger amplitude, the revival time shifts to smaller values. The dashed line corresponds to a theory including a higher order interaction term $\beta a^\dagger a^\dagger aa|e\rangle\langle e|$ in the Hamiltonian, with $\beta = -23$ kHz. **d,** Predicted signal $S$ as a function of both delay time $\tau$ and displacement amplitude $\alpha$. It is obtained using a simple theory without higher order interaction term (Eq. S23). Lines show cuts from **b**.

[1] P. Facchi, V. Gorini, G. Marmo, S. Pascazio and E. C. G. Sudarshan. Quantum Zeno dynamics. *Phys. Lett. A* 12–19 (2000).
[2] P. Facchi and S. Pascazio. Quantum Zeno Subspaces. *Phys. Rev. Lett.* **89**, 080401 (2002).
[3] P. Facchi, D. Lidar and S. Pascazio. Unification of dynamical decoupling and the quantum Zeno effect. *Phys. Rev. A* **69**, 032314 (2004).
[4] J. M. Raimond, C. Sayrin, S. Gleyzes, I. Dotsenko, M. Brune, S. Haroche, P. Facchi and S. Pascazio. Phase Space Tweezers for Tailoring Cavity Fields by Quantum Zeno Dynamics. *Phys. Rev. Lett.* **105**, 213601 (2010).
[5] J. M. Raimond, P. Facchi, B. Peaudecerf, S. Pascazio, C. Sayrin, I. Dotsenko, S. Gleyzes, M. Brune and S. Haroche. Quantum Zeno dynamics of a field in a cavity. *Phys. Rev. A* **86**, 032120 (2012).
[6] B. Misra and E. C. G. Sudarshan. The Zeno's paradox in quantum theory. *J. Math. Phys.* **18**, 756 (1977).
[7] Originally, QZD corresponded to quantum evolutions restricted by measurement. Yet, the name was later extended to any quantum dynamics in a restricted Hilbert space [3].
[8] F. Schäfer, I. Herrera, S. Cherukattil, C. Lovecchio, F. S. Cataliotti, F. Caruso and A. Smerzi. Experimental realization

of quantum zeno dynamics. *Nat. Commun.* **5**, 3194 (2014).

[9] A. Signoles, A. Facon, D. Grosso, I. Dotsenko, S. Haroche, J.-M. Raimond, M. Brune and S. Gleyzes. Confined quantum Zeno dynamics of a watched atomic arrow. *Nat. Phys.* **10**, 715–719 (2014).

[10] D. I. Schuster, A. A. Houck, J. A. Schreier, A. Wallraff, J. M. Gambetta, A. Blais, L. Frunzio, J. Majer, B. Johnson, M. H. Devoret, S. M. Girvin and R. J. Schoelkopf. Resolving photon number states in a superconducting circuit. *Nature* **445**, 515–8 (2007).

[11] H. Paik, D. I. Schuster, L. S. Bishop, G. Kirchmair, G. Catelani, A. P. Sears, B. R. Johnson, M. J. Reagor, L. Frunzio, L. I. Glazman, S. M. Girvin, M. H. Devoret and R. J. Schoelkopf. Observation of High Coherence in Josephson Junction Qubits Measured in a Three-Dimensional Circuit QED Architecture. *Phys. Rev. Lett.* **107**, 240501 (2011).

[12] G. Kirchmair, B. Vlastakis, Z. Leghtas, S. E. Nigg, H. Paik, E. Ginossar, M. Mirrahimi, L. Frunzio, S. M. Girvin and R. J. Schoelkopf. Observation of quantum state collapse and revival due to the single-photon Kerr effect. *Nature* **495**, 205–9 (2013).

[13] Materials and methods are available as supplementary material on Science Online.

[14] S. E. Nigg, H. Paik, B. Vlastakis, G. Kirchmair, S. Shankar, L. Frunzio, M. H. Devoret, R. J. Schoelkopf and S. M. Girvin. Black-Box Superconducting Circuit Quantization. *Phys. Rev. Lett.* **108**, 240502 (2012).

[15] J. Bourassa, F. Beaudoin, J. M. Gambetta and a. Blais. Josephson-junction-embedded transmission-line resonators: From Kerr medium to in-line transmon. *Phys. Rev. A* **86**, 013814 (2012).

[16] F. Solgun, D. W. Abraham and D. P. DiVincenzo. Blackbox quantization of superconducting circuits using exact impedance synthesis. *Phys. Rev. B* **90**, 134504 (2014).

[17] L. Lutterbach and L. Davidovich. Method for Direct Measurement of the Wigner Function in Cavity QED and Ion Traps. *Phys. Rev. Lett.* **78**, 2547–2550 (1997).

[18] P. Bertet, a. Auffeves, P. Maioli, S. Osnaghi, T. Meunier, M. Brune, J. Raimond and S. Haroche. Direct Measurement of the Wigner Function of a One-Photon Fock State in a Cavity. *Phys. Rev. Lett.* **89**, 200402 (2002).

[19] B. Vlastakis, G. Kirchmair, Z. Leghtas, S. E. Nigg, L. Frunzio, S. M. Girvin, M. Mirrahimi, M. H. Devoret and R. J. Schoelkopf. Deterministically encoding quantum information using 100-photon Schrödinger cat states. *Science* **342**, 607–10 (2013).

[20] S. Haroche and J.-M. Raimond. *Exploring the Quantum: Atoms, Cavities, and Photons* (Oxford Graduate Texts, 2006).

[21] S. Maniscalco, F. Francica, R. L. Zaffino, N. Lo Gullo and F. Plastina. Protecting Entanglement via the Quantum Zeno Effect. *Phys. Rev. Lett.* **100**, 090503 (2008).

[22] X.-B. Wang, J. Q. You and F. Nori. Quantum entanglement via two-qubit quantum Zeno dynamics. *Phys. Rev. A* **77**, 062339 (2008).

[23] Z. C. Shi, Y. Xia, H. Z. Wu and J. Song. One-step preparation of three-particle Greenberger-Horne-Zeilinger state via quantum Zeno dynamics. *Eur. Phys. J. D* **66**, 127 (2012).

[24] X.-Q. Shao, L. Chen, S. Zhang and K.-H. Yeon. Fast CNOT gate via quantum Zeno dynamics. *J. Phys. B At. Mol. Opt. Phys.* **42**, 165507 (2009).

[25] M. Mirrahimi, Z. Leghtas, V. V. Albert, S. Touzard, R. J. Schoelkopf, L. Jiang and M. H. Devoret. Dynamically protected cat-qubits: a new paradigm for universal quantum computation. *New J. Phys.* **16**, 045014 (2014).

[26] N. Roch, E. Flurin, F. Nguyen, P. Morfin, P. Campagne-Ibarcq, M. H. Devoret and B. Huard. Widely Tunable, Non-degenerate Three-Wave Mixing Microwave Device Operating near the Quantum Limit. *Phys. Rev. Lett.* **108**, 147701 (2012).

[27] The thermalization of the qubit and of the cavity are very different in nature because the qubit is quite thermally isolated on a sapphire chip poorly anchored inside the superconducting cavity. By looking at the spectroscopy of the qubit (Fig. S2d), one can estimate a thermal occupation of the cavity smaller than 0.04.

[28] J. Gambetta, A. Blais, D. Schuster, a. Wallraff, L. Frunzio, J. Majer, M. Devoret, S. Girvin and R. Schoelkopf. Qubit-photon interactions in a cavity: Measurement-induced dephasing and number splitting. *Phys. Rev. A* **74**, 042318 (2006).

[29] In the initial cool-down, the parameters were $f_c = 7.8041$ GHz, $f_q = 5.624$ GHz, $\alpha = 170$ MHz and $\chi = 5.35$ MHz. Although not quantitatively extracted in this run, $\lambda$ was measured as positive from measurements similar as Fig. S2c-d, in the range of few tens of kHz. Using the formulae from the pure transmon case [14], the Kerr frequency can be estimated as $\lambda = \chi^2/(4\alpha) =$ 42 kHz, which is compatible with these measurements.

[30] J. Johansson, P. Nation and F. Nori. QuTiP 2: A Python framework for the dynamics of open quantum systems. *Comput. Phys. Commun.* **184**, 1234–1240 (2013).

[31] K. Geerlings, Z. Leghtas, I. Pop, S. Shankar, L. Frunzio, R. Schoelkopf, M. Mirrahimi and M. Devoret. Demonstrating a Driven Reset Protocol for a Superconducting Qubit. *Phys. Rev. Lett.* **110**, 120501 (2013).

[32] F. Motzoi, J. Gambetta, P. Rebentrost and F. Wilhelm. Simple Pulses for Elimination of Leakage in Weakly Nonlinear Qubits. *Phys. Rev. Lett.* **103**, 110501 (2009).
